# Supplementary material for: Are Self-Driving Cars Secure? Evasion Attacks against Deep Neural Networks for Steering Angle Prediction
Source: arXiv:1904.07370 source file (2019-04-15)
Supplement: Supplementary file 1 [file appendix.tex]

\section{Adversarial images}

In Figure~\ref{fig:exepoch} we show examples of original images (on the left), and two corresponding adversarial images in the center and left for the Epoch model. Similarly we show adversarial images for the NVIDIA model in Figure~\ref{fig:exnvidia}. We thus demonstrate that adversarial images can be created from any original class to any targeted class.  

\begin{figure*}
\centering
\begin{subfigure}[t]{0.6\columnwidth}
\includegraphics[width=\columnwidth]{images/epoch/center.png}
\caption{Input image,  'straight'}
\end{subfigure}
\begin{subfigure}[t]{0.6\columnwidth}
\includegraphics[width=\columnwidth]{images/epoch/centerleft.png}
\caption{Adversarial image, 'left'}
\end{subfigure}
\begin{subfigure}[t]{0.6\columnwidth}
\includegraphics[width=\columnwidth]{images/epoch/centerright.png}
\caption{Adversarial image, 'right'}
\end{subfigure}

\begin{subfigure}[t]{0.6\columnwidth}
\includegraphics[width=\columnwidth]{images/epoch/left.png}
\caption{Input image,  'left'}
\end{subfigure}
\begin{subfigure}[t]{0.6\columnwidth}
\includegraphics[width=\columnwidth]{images/epoch/leftcenter.png}
\caption{Adversarial image, 'straight'}
\end{subfigure}
\begin{subfigure}[t]{0.6\columnwidth}
\includegraphics[width=\columnwidth]{images/epoch/leftright.png}
\caption{Adversarial image, 'right'}
\end{subfigure}

\begin{subfigure}[t]{0.6\columnwidth}
\includegraphics[width=\columnwidth]{images/epoch/right.png}
\caption{Input image,  'right'}
\end{subfigure}
\begin{subfigure}[t]{0.6\columnwidth}
\includegraphics[width=\columnwidth]{images/epoch/rightcenter.png}
\caption{Adversarial image, 'straight'}
\end{subfigure}
\begin{subfigure}[t]{0.6\columnwidth}
\includegraphics[width=\columnwidth]{images/epoch/rightleft.png}
\caption{Adversarial image, 'left'}
\end{subfigure}
\caption{Adversarial images for the Epoch model}
\label{fig:exepoch}
\end{figure*}

\begin{figure*}
\centering
\begin{subfigure}[t]{0.6\columnwidth}
\includegraphics[width=\columnwidth]{images/nvidia/straight.png}
\caption{Input image,  'straight'}
\end{subfigure}
\begin{subfigure}[t]{0.6\columnwidth}
\includegraphics[width=\columnwidth]{images/nvidia/straightleft.png}
\caption{Adversarial image, 'left'}
\end{subfigure}
\begin{subfigure}[t]{0.6\columnwidth}
\includegraphics[width=\columnwidth]{images/nvidia/straightright.png}
\caption{Adversarial image, 'right'}
\end{subfigure}

\begin{subfigure}[t]{0.6\columnwidth}
\includegraphics[width=\columnwidth]{images/nvidia/left.png}
\caption{Input image,  'left'}
\end{subfigure}
\begin{subfigure}[t]{0.6\columnwidth}
\includegraphics[width=\columnwidth]{images/nvidia/leftstraight.png}
\caption{Adversarial image, 'straight'}
\end{subfigure}
\begin{subfigure}[t]{0.6\columnwidth}
\includegraphics[width=\columnwidth]{images/nvidia/leftright.png}
\caption{Adversarial image, 'right'}
\end{subfigure}

\begin{subfigure}[t]{0.6\columnwidth}
\includegraphics[width=\columnwidth]{images/nvidia/right.png}
\caption{Input image,  'right'}
\end{subfigure}
\begin{subfigure}[t]{0.6\columnwidth}
\includegraphics[width=\columnwidth]{images/nvidia/rightstraight.png}
\caption{Adversarial image, 'straight'}
\end{subfigure}
\begin{subfigure}[t]{0.6\columnwidth}
\includegraphics[width=\columnwidth]{images/nvidia/rightleft.png}
\caption{Adversarial image, 'left'}
\end{subfigure}
\caption{Adversarial images for the NVIDIA model}
\label{fig:exnvidia}
\end{figure*}
